# Supplementary material for: PointMixer: MLP-Mixer for Point Cloud Understanding
Source: arXiv:2111.11187 source file (2022-07-20)
Supplement: Supplementary file 1 [file supp_t1_robustness.tex]

\begin{table}[!t]
\caption{Robustness experiments with random noises. 
% `PT' and `PM' denote Point Transformer and PointMixer, respectively.
}
\vspace{-3.5mm}
\label{table:rebuttal-robustness}
\centering
\resizebox{\linewidth}{!}{
\begin{tabular}{l|c|c|cc}
\toprule
& Add noise & \multicolumn{1}{c|}{Semseg (S3DIS)} & \multicolumn{2}{c}{Classification (ModelNet40)} \\ 
& ($\sigma{=}0.01$) & mIoU $(\%)$ & mAcc $(\%)$ & OA $(\%)$ \\
\midrule

\rowcolor{gray!20} PointTransformer$^{\textcolor{red}{3}}$ & & 70.0~~~~~~~~~~~~~~ & 91.1~~~~~~~~~~~~ & 93.3~~~~~~~~~~~~ \\

& \checkmark & 55.5 (\textcolor{purple}{$\downarrow$ 14.5}) & 89.9 (\textcolor{purple}{$\downarrow$ 1.2}) & 92.4 (\textcolor{purple}{$\downarrow$ 0.9}) \\

\midrule

\rowcolor{yellow!20} PointMixer (ours) & & 71.4~~~~~~~~~~~~~~ & 91.4~~~~~~~~~~~~~& 93.6~~~~~~~~~~~~~\\

& \checkmark & 58.7 (\textcolor{purple}{$\downarrow$ 12.7}) & 91.0 (\textcolor{purple}{$\downarrow$ 0.4}) & 92.7 (\textcolor{purple}{$\downarrow$ 0.9}) \\

% \multirow{3}{*}[-0.5ex]{PointTransformer} & \redxmark & - & 70.4 \\
% & \greencheck~(max) &  & (running) \\
% & \greencheck~(softmax) &  & (running) \\
% \midrule
% PointMixer (ours) & \greencheck~(softmax) & - & 71.4 \\
\bottomrule
\end{tabular}
}
\vspace{-4mm}
\end{table}
