# Supplementary material for: PointMixer: MLP-Mixer for Point Cloud Understanding
Source: arXiv:2111.11187 source file (2022-07-20)
Supplement: Supplementary file 2 [file supp_t2_comparison.tex]

% \begin{wraptable}{r}{0.60\textwidth}
\begin{table}[!t]
\centering
\caption{Technical comparisons.}
\vspace{-3mm}
\resizebox{1.00\linewidth}{!}{
\begin{tabular}{lcccccc}

\Xhline{4\arrayrulewidth} 

\multirow{2}{*}[-0.5ex]{Method} & \multirow{2}{*}[-0.5ex]{~~~Locality~~~} & \multicolumn{3}{c}{~Set operator~} & ~~~Symmetric~~~ & \multirow{2}{*}[-0.5ex]{~Token-mix~} 
\\ \cline{3-5}

 &  & Intra & ~Inter~ & Hier & pyramid arch & 
\\ \Xhline{2\arrayrulewidth}

PointNet\plusplus & \greencheck & \greencheck & \redxmark & \redxmark & \redxmark & Pooling 
\\ 

PointConv & \greencheck & \greencheck & \redxmark & \redxmark & \redxmark & Conv
\\ 

PointTrans & \greencheck & \greencheck & \redxmark & \redxmark & \redxmark & Self-attn 
\\ 

\rowcolor{yellow!20} PointMixer & \greencheck & \greencheck & \greencheck & \greencheck & \greencheck & Softmax 
\\ \Xhline{4\arrayrulewidth} 

\end{tabular}
}
% \label{table:compare}
\end{table}
